# Supplementary material for: GrounDial: Human-norm Grounded Safe Dialog Response Generation
Source: arXiv:2402.08968 source file (2024-02-14)
Supplement: Supplementary file 1 [file A_Appendix.tex]

\section{Related Works}
% \subsection{Safe Response Generation with Additional Tuning} 
Conventional approaches for safe dialog systems mostly focused on collecting exemplary safe dialogue samples and fine-tuning a pre-trained LLM on them. 
Earlier approaches~\cite{ung2021saferdialogues, kim2022prosocialdialog, ziems2022moral} used crowd-sourcing platforms such as Amazon Mechanical Turk to manually collect safe responses from human annotators. 
More recent approaches collected RoT along with safe dialogues and fine-tuned the LLM to generate response and relevant RoT at the same time~\cite{kim2022prosocialdialog, sun2023moraldial}.

On the other hand, decoding-based approaches do not directly fine-tune the LLM.
However, it still requires additional datasets and tuning to prepare an auxiliary safety classifier, namely discriminator~\cite{krause2021gedi} or experts~\cite{liu2021dexperts, hallinan2022detoxifying} 
The pre-trained classifier is used to determine if the responses generated until a certain decoding step is safe or not. 
In contrast, GrounDial does not necessitate additional training of the LLM.

% \subsection{Without additional tuning}
There is a lack of safe response generation research that mitigates the dependency on tuning. 
To the best of our knowledge, there is only one such paper that proposed in-context learning of safe dialogues from~\cite{meade2023using}. 
Specifically, it retrieves several dialog examples from pre-collected safe dialogue histories and appends them to the current user input, so that the agent can be guided to follow the safe examples. 
However, although it did not perform fine-tuning, it still relies on manually collected safe dialogues for retrieval.

\section{Experimental Details}
% \subsection{ProsocialDialog Dataset}
\subsection{Details of HGD}
For HGD implementation, we used the official code of knowledge infused decoding (KID)~\cite{liu2022knowledge}~\footnote{\url{https://github.com/microsoft/KID.git}}. 

\subsection{Safety Classifiers}
We adopted pre-trained safety classifiers provided by ParlAI~\cite{miller2017parlai}.
In particular, we chose the three most widely used classifiers, \path{zoo:dialogue_safety/single_turn/model}, \path{bot_adversarial_dialogue/multi_turn_v0/model}, and \path{bot_adversarial_dialogue/multi_turn/model}.
They are based on RoBERTa architecture and the classification head was fine-tuned with ground-truth (context, response, safety labels) pairs. 

\section{Additional Evaluation}
\subsection{LLM-aided Evaluation}
Recent LLM with advanced language understanding capability can serve as a reliable safety classifier. 
In other words, when given a dialog history and response, it can detect if the response is safe or not. 
Therefore, we additionally conducted an LLM-aided evaluation for a more faithful comparison. 

Our first attempt to instruct ChatGPT~\footnote{\url{https://chat.openai.com/}} to work as a safety classifier, i.e., ``Now you are a binary classifier that classifies given response is safe or not'', assign ``safe'' label too generously.
In other words, it annotated neutral or off-topic responses as ``safe'' which is not desirable. 
Therefore, we conducted a paired comparison between the GrounDial and baselines using the prompt written below. 
\begin{minted}
[
frame=lines,
framesep=2mm,
baselinestretch=1.2,
% bgcolor=LightGray,
fontsize=\footnotesize,
linenos,
breaklines
]
{python}
prompt = "Whose answer expresses more concern and discourage User? Agent A or B?"
\end{minted}
The responses to the same context from GrounDial and baseline were appended to the prompt, each specified as either Agent A or B.

The Table~\ref{tab::llm} shows the results of the LLM-aided evaluation. 
It displays the winning ratio of the method marked in bold in the leftmost column. 
Notably, 71.54\% of the responses are classified as safer than vanilla Blenderbot, which clearly supports the effectiveness of GrounDial in improving response safety. 
\begin{table}[h!]
\centering
\begin{tabular}{cc}
\toprule
& \multicolumn{1}{l}{\textbf{Winning ratio}} \\
\midrule
Vanilla vs. \textbf{Ours}                  & 71.54\%                                    \\
Fine-tuned vs. \textbf{Ours}               & 40.02\%                                    \\
Fine-tuned vs. \textbf{Vanilla}            & 29.06\% \\
\bottomrule
\end{tabular}
\caption{LLM-aided evaluation result}
\label{tab::llm}
\end{table}

\begin{table*}[ht!]
\centering
\begin{tabular}{l|cc|ccccc}
\toprule
& \multicolumn{2}{c|}{\textbf{Retrieval precision}}                          & \multicolumn{5}{c}{\textbf{Agreement acc.}}                                                                                                                                       \\
\multirow{-2}{*}{\textbf{Embedding}} & {Prec@1}                     & \multicolumn{1}{c|}{{Prec@3}} & None & {Random}                              & \multicolumn{1}{c}{{Top-1}} & \multicolumn{1}{c}{{Top-3}} & \multicolumn{1}{c}{{GT}} \\
\midrule
\textbf{SimCSE}                                                             & \multicolumn{1}{r}{0.0981}          & 0.1549                                                      & & \multicolumn{1}{r}{}                         & 0.3960                                                     & 0.3881                                                     &                                                         \\
\textbf{MPNet}                                                              & \multicolumn{1}{r}{\textbf{0.1909}} & {\textbf{0.2844}}                      & \multicolumn{1}{r}{\multirow{-2}{*}{0.3200}}                  & \multicolumn{1}{r}{\multirow{-2}{*}{0.3366}} & \textbf{0.4345}                                            & \textbf{0.4638}                                            & \multirow{-2}{*}{0.4970}                               \\
\bottomrule
\end{tabular}
\caption{Retrieval performance and agreement score for various retrieval numbers}
\label{tab::embedding_space}
\end{table*}

\subsection{Analysis on RoT Retrieval}
Accurate retrieval of relevant RoT is essential for generating appropriately grounded responses.
For a deeper analysis of the effect of RoT retrieval, we conducted additional experiments with various RoT selection schemes.
The agreement scores from different schemes are shown in Table~\ref{tab::embedding_space}.
Regardless of the selection scheme, the scores were measured with the ground truth RoTs. 

First, we measured the RoT agreement score of the responses generated by grounding to \textit{randomly} selected RoTs from the pre-defined RoT set.
It is denoted as Random in the table. 
The result of random RoT selection is similar to that of None which indicates not using RoT.
On the other hand, when the responses are grounded in the ground truth (GT) RoTs, the agreement score increases significantly. 
It can be implied that grounding to RoT is effective but grounding to \textit{any} RoT is not useful; it underscores the importance of selecting and injecting relevant RoTs. 
The retrieved RoTs show superior results than Random results, suggesting that if the RoTs become more accurate, then the agreement score will further improve.
This indicates that the sentence embedding modules can cluster related context and RoT closely.

To test this hypothesis, we experimented with an additional sentence embedding space, SimCSE~\cite{gao2021simcse}.
It was proposed before MPNet that we have used throughout experiments and is known to have weaker representational power than MPNet. 
This can also be measured by retrieval precision shown in the left columns in Table~\ref{tab::embedding_space}.

As shown in the table, the retrieval precision for the top-3 increases compared to top-1. 
This indicates that even if the exact RoT is not retrieved, there is a higher possibility that the ground-truth RoT is included in top-3 retrieved RoTs. 
This is also reflected in the agreement score of using MPNet, where the score increases when the top-3 retrieved RoT are injected. 
In addition, as the retrieval precision improves by moving from SimCSE to MPNet, the agreement score also increases. 
This indicates that replacing the sentence embedding module with a more improved LLM can potentially bring more performance gain. 

% \section{Ablation Study}
% % \subsection{Effect of Retrieval Number}
% \subsection{Effect of Hyper-parameters}
% In this section, we examine the effect of two primary hyper-parameters, 
% $\beta$ that scales KL divergence in policy update and the number of steps of update.

% \subsection{Effect of Prompt}
% \input{Table/prompt_exploration}
% We explored the effect of different prompt template on the generated responses.
% Specifically, we tried four types of templates as below:

% The results are shown in Table~\ref{tab::prompts}.
% It is shown that for BBot, simple concatenation in front of input context is most effective to improve both safety score and agreement score. 

% \subsection{ICL Prompting Exploration}
